# Supplementary material for: Can co-location be used as a proxy for face-to-face contacts?
Source: arXiv:1712.06346 ancillary file (2017-12-18)
Supplement: Supplementary file 1 [file article_v5_SI.pdf]

**Supplementary information**  
**for**  
**Can co-location be used as a proxy for face-to-face contacts?**

Mathieu Génois\*

*Aix Marseille Univ, Université de Toulon, CNRS, CPT, Marseille, France and  
GESIS, Leibniz Institute for the Social Sciences,  
Unter Sachsenhausen 6-8, 50667 Köln, Germany*

Alain Barrat

*Aix Marseille Univ, Université de Toulon, CNRS, CPT, Marseille, France and  
Data Science Laboratory, ISI Foundation, Torino, Italy*

(Dated: December 18, 2017)

---

\* mathieu.genois@gesis.org

|                                                           |             | InVS13             | InVS15             | LH10               | LyonSchool         | SFHH               | Thiers13           |
|-----------------------------------------------------------|-------------|--------------------|--------------------|--------------------|--------------------|--------------------|--------------------|
| $\langle w \rangle$                                       | Contact     | 8.17               | 6.89               | 20.3               | 9.14               | 5.77               | 20.2               |
|                                                           | Co-presence | 79.6               | 47.9               | 46.3               | 226                | 17.5               | 339                |
|                                                           | Sampling 1  | 6.50               | 8.68               | 29.1               | 7.54               | 2.19               | 10.3               |
|                                                           | Sampling 2  | 30.6               | 27.9               | 48.1               | 17.9               | 5.44               | 48.1               |
|                                                           | Sampling 3  | 5.60               | 17.8               | 29.8               | 27.3               | 5.61               | 56.7               |
| $\langle w^2 \rangle$                                     | Contact     | $1.53 \times 10^3$ | $6.93 \times 10^3$ | $1.02 \times 10^4$ | 834                | 545                | $1.05 \times 10^5$ |
|                                                           | Co-presence | $7.85 \times 10^4$ | $3.42 \times 10^4$ | $4.39 \times 10^4$ | $1.51 \times 10^5$ | $1.22 \times 10^3$ | $6.99 \times 10^5$ |
|                                                           | Sampling 1  | 264                | $1.13 \times 10^3$ | $8.93 \times 10^3$ | 174                | 14.8               | 259                |
|                                                           | Sampling 2  | $6.30 \times 10^3$ | $2.49 \times 10^4$ | $3.54 \times 10^4$ | $1.19 \times 10^3$ | 526                | $1.02 \times 10^4$ |
|                                                           | Sampling 3  | 271                | $4.26 \times 10^3$ | $6.80 \times 10^3$ | $1.18 \times 10^4$ | 221                | $5.35 \times 10^4$ |
| $\frac{\langle w^2 \rangle}{\langle w \rangle}$           | Contact     | 187                | 67.7               | 341                | 91.3               | 94.6               | 521                |
|                                                           | Co-presence | 986                | 714                | 947                | 669                | 69.5               | $2.06 \times 10^3$ |
|                                                           | Sampling 1  | 40.7               | 130                | 306                | 23.1               | 6.77               | 25.2               |
|                                                           | Sampling 2  | 206                | 893                | 736                | 66.4               | 96.7               | 211                |
|                                                           | Sampling 3  | 48.4               | 239                | 228                | 433                | 39.5               | 944                |
| $\langle n \rangle$                                       | Contact     | 4.02               | 3.63               | 8.87               | 6.01               | 2.77               | 7.71               |
|                                                           | Co-presence | 33.4               | 18.6               | 17.6               | 67.4               | 10.4               | 70.4               |
|                                                           | Sampling 1  | 6.27               | 7.80               | 22.4               | 7.22               | 2.05               | 10.0               |
|                                                           | Sampling 2  | 1.77               | 2.50               | 5.03               | 2.12               | 1.36               | 1.32               |
|                                                           | Sampling 3  | 2.32               | 1.59               | 11.0               | 1.36               | 1.17               | 1.20               |
| $\langle n^2 \rangle$                                     | Contact     | 172                | 62.4               | 478                | 207                | 65.5               | 677                |
|                                                           | Co-presence | $6.81 \times 10^3$ | $2.56 \times 10^3$ | $3.27 \times 10^3$ | $1.62 \times 10^5$ | 282                | $2.65 \times 10^5$ |
|                                                           | Sampling 1  | 242                | 835                | $4.45 \times 10^3$ | 155                | 12.0               | 242                |
|                                                           | Sampling 2  | 5.76               | 26.4               | 126                | 7.54               | 3.09               | 2.18               |
|                                                           | Sampling 3  | 14.1               | 4.24               | 474                | 2.34               | 1.62               | 1.69               |
| $\frac{\langle n^2 \rangle}{\langle n \rangle}$           | Contact     | 42.8               | 17.2               | 53.9               | 34.5               | 23.6               | 87.8               |
|                                                           | Co-presence | 204                | 137                | 185                | 240                | 27.0               | 376                |
|                                                           | Sampling 1  | 38.5               | 107                | 199                | 21.5               | 5.88               | 24.1               |
|                                                           | Sampling 2  | 3.26               | 10.6               | 25.1               | 3.55               | 2.28               | 1.65               |
|                                                           | Sampling 3  | 6.07               | 2.66               | 43.1               | 1.71               | 1.38               | 1.40               |
| $\langle \tau_c \rangle$                                  | Contact     | 2.03               | 1.90               | 2.29               | 1.52               | 2.08               | 2.61               |
|                                                           | Co-presence | 2.39               | 2.59               | 2.66               | 3.36               | 1.68               | 4.81               |
|                                                           | Sampling 1  | 1.04               | 1.11               | 1.30               | 1.04               | 1.07               | 1.02               |
|                                                           | Sampling 2  | 17.3               | 11.2               | 9.57               | 8.44               | 4.02               | 36.3               |
|                                                           | Sampling 3  | 2.42               | 11.2               | 2.71               | 20.0               | 4.79               | 47.2               |
| $\langle \tau_c^2 \rangle$                                | Contact     | 84.1               | 22.5               | 15.6               | 6.02               | 16.2               | 48.4               |
|                                                           | Co-presence | 58.1               | 38.4               | 66.3               | 53.0               | 13.6               | 227                |
|                                                           | Sampling 1  | 1.11               | 1.38               | 2.14               | 1.14               | 1.21               | 1.08               |
|                                                           | Sampling 2  | $2.25 \times 10^3$ | 829                | 898                | 350                | 212                | $6.22 \times 10^3$ |
|                                                           | Sampling 3  | 60.8               | $2.30 \times 10^3$ | 67.2               | $8.50 \times 10^3$ | 177                | $4.37 \times 10^4$ |
| $\frac{\langle \tau_c^2 \rangle}{\langle \tau_c \rangle}$ | Contact     | 41.4               | 11.9               | 6.81               | 3.96               | 7.79               | 18.5               |
|                                                           | Co-presence | 24.3               | 14.8               | 24.9               | 15.8               | 8.09               | 47.1               |
|                                                           | Sampling 1  | 1.07               | 1.23               | 1.65               | 1.09               | 1.14               | 1.05               |
|                                                           | Sampling 2  | 130                | 74.1               | 93.8               | 41.5               | 52.7               | 171                |
|                                                           | Sampling 3  | 25.2               | 206                | 24.8               | 425                | 37.0               | 926                |
| $\langle \tau_i \rangle$                                  | Contact     | $1.03 \times 10^3$ | $1.50 \times 10^3$ | 282                | 333                | 159                | 534                |
|                                                           | Co-presence | 495                | 609                | 78.8               | 52.7               | 245                | 93.8               |
|                                                           | Sampling 1  | $2.14 \times 10^3$ | $1.54 \times 10^3$ | 131                | 392                | 658                | 907                |
|                                                           | Sampling 2  | $7.43 \times 10^3$ | $4.22 \times 10^3$ | 472                | $1.26 \times 10^3$ | 865                | $5.22 \times 10^3$ |
|                                                           | Sampling 3  | $5.74 \times 10^3$ | $8.37 \times 10^3$ | 276                | $1.89 \times 10^3$ | $1.33 \times 10^3$ | $5.20 \times 10^3$ |
| $\langle \tau_i^2 \rangle$                                | Contact     | $2.50 \times 10^7$ | $3.24 \times 10^7$ | $9.95 \times 10^5$ | $1.04 \times 10^6$ | $4.62 \times 10^5$ | $3.94 \times 10^6$ |
|                                                           | Co-presence | $1.01 \times 10^7$ | $1.17 \times 10^7$ | $2.23 \times 10^5$ | $1.32 \times 10^5$ | $6.45 \times 10^5$ | $5.70 \times 10^5$ |
|                                                           | Sampling 1  | $4.45 \times 10^7$ | $3.17 \times 10^7$ | $4.00 \times 10^5$ | $1.05 \times 10^6$ | $1.99 \times 10^6$ | $4.83 \times 10^6$ |
|                                                           | Sampling 2  | $1.59 \times 10^8$ | $8.60 \times 10^7$ | $1.60 \times 10^6$ | $4.22 \times 10^6$ | $2.63 \times 10^6$ | $4.98 \times 10^7$ |
|                                                           | Sampling 3  | $1.43 \times 10^8$ | $2.05 \times 10^8$ | $8.56 \times 10^5$ | $7.03 \times 10^6$ | $4.30 \times 10^6$ | $5.23 \times 10^7$ |
| $\frac{\langle \tau_i^2 \rangle}{\langle \tau_i \rangle}$ | Contact     | $2.44 \times 10^4$ | $2.16 \times 10^4$ | $3.52 \times 10^3$ | $3.12 \times 10^3$ | $2.89 \times 10^3$ | $7.38 \times 10^3$ |
|                                                           | Co-presence | $2.04 \times 10^4$ | $1.92 \times 10^4$ | $2.83 \times 10^3$ | $2.51 \times 10^3$ | $2.63 \times 10^3$ | $6.08 \times 10^3$ |
|                                                           | Sampling 1  | $2.08 \times 10^4$ | $2.06 \times 10^4$ | $3.05 \times 10^3$ | $2.69 \times 10^3$ | $3.03 \times 10^3$ | $5.33 \times 10^3$ |
|                                                           | Sampling 2  | $2.14 \times 10^4$ | $2.04 \times 10^4$ | $3.40 \times 10^3$ | $3.34 \times 10^3$ | $3.04 \times 10^3$ | $9.55 \times 10^3$ |
|                                                           | Sampling 3  | $2.48 \times 10^4$ | $2.45 \times 10^4$ | $3.10 \times 10^3$ | $3.73 \times 10^3$ | $3.23 \times 10^3$ | $1.01 \times 10^4$ |

TABLE I. **Comparison of the moments of the temporal distributions between the contact and the co-presence events.** For each dataset we compute the first and second moment of the distributions of link weights, event frequencies, event durations and inter-event durations, along with the ratio of the two.

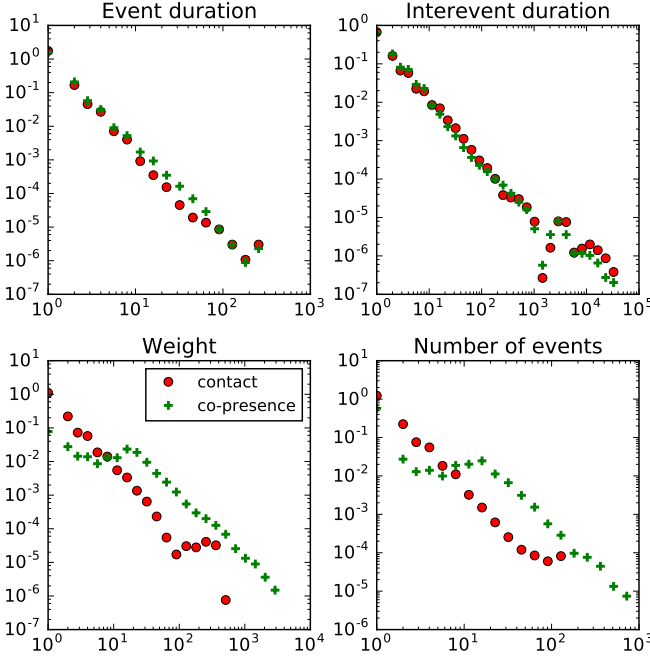

FIG. 1. Temporal distributions for co-presence and contact events — InVS13. We show for both the contact and co-presence of the same data set the distributions of event and inter-event duration, link weights (as total contact duration) and number of contacts per link.

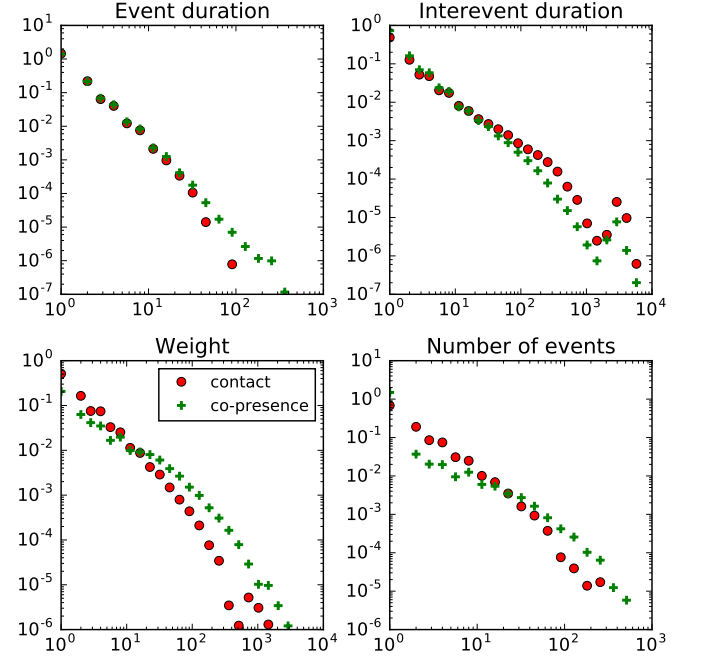

FIG. 2. Temporal distributions for co-presence and contact events — LH10. We show for both the contact and co-presence of the same data set the distributions of event and inter-event duration, link weights (as total contact duration) and number of contacts per link.

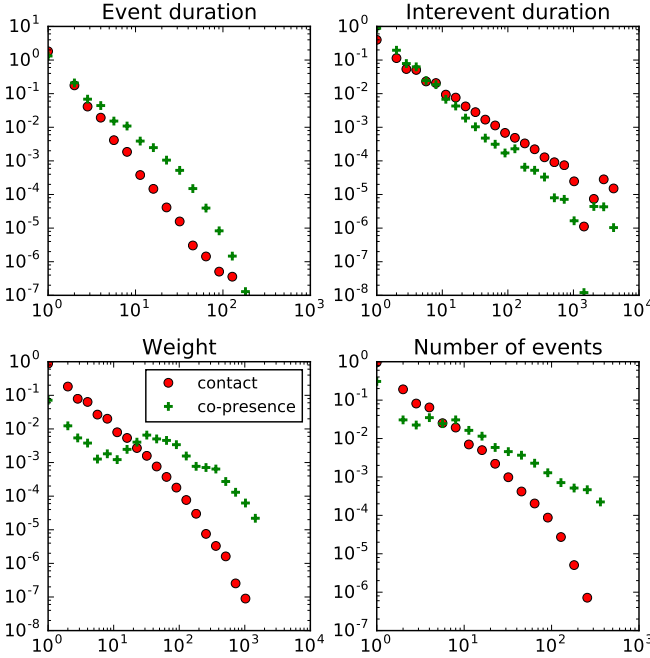

FIG. 3. Temporal distributions for co-presence and contact events — LyonSchool. We show for both the contact and co-presence of the same data set the distributions of event and inter-event duration, link weights (as total contact duration) and number of contacts per link.

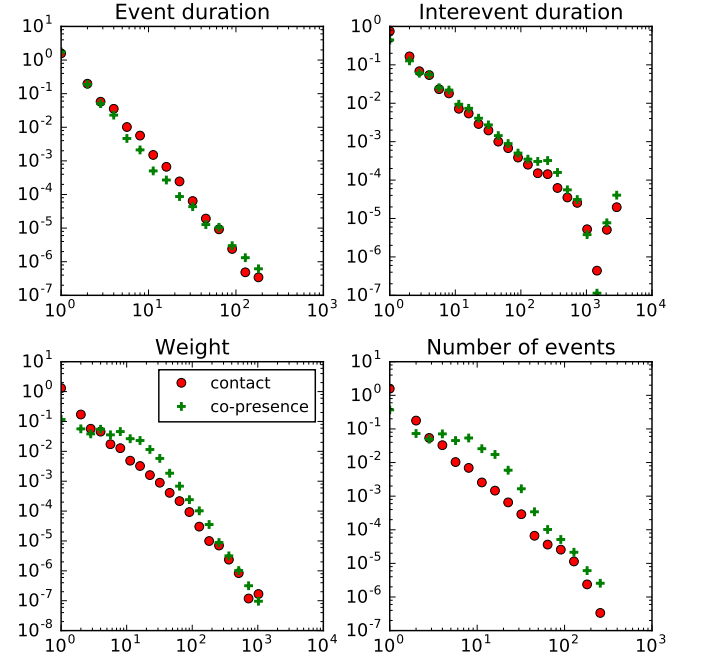

FIG. 4. Temporal distributions for co-presence and contact events — SFHH. We show for both the contact and co-presence of the same data set the distributions of event and inter-event duration, link weights (as total contact duration) and number of contacts per link.

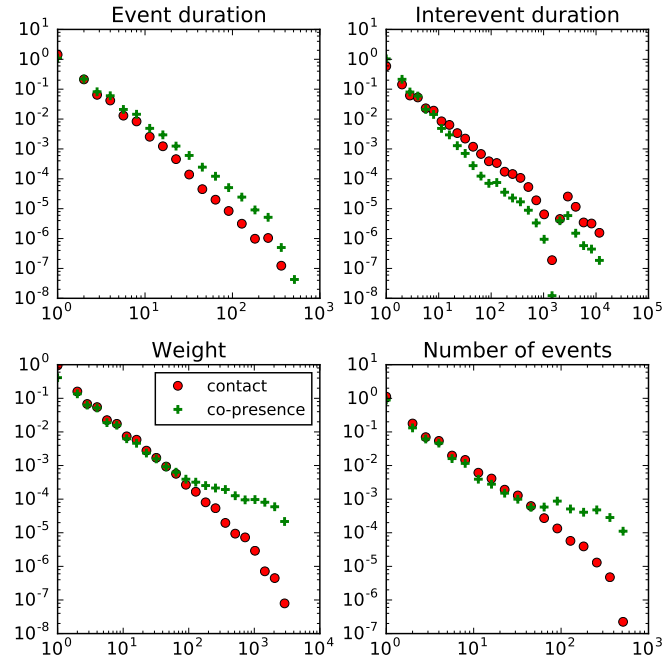

FIG. 5. **Temporal distributions for co-presence and contact events — Thiers13.** We show for both the contact and co-presence of the same data set the distributions of event and inter-event duration, link weights (as total contact duration) and number of contacts per link.

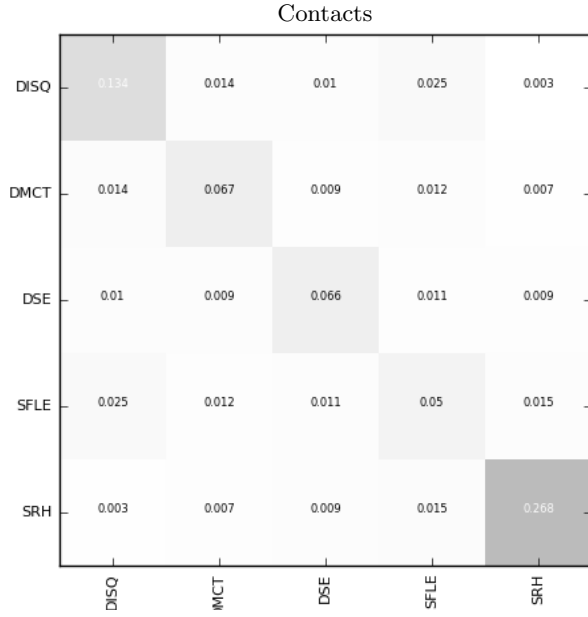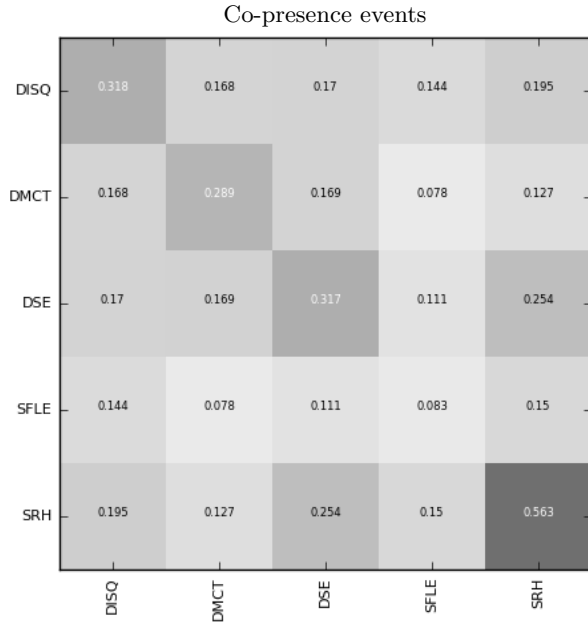

FIG. 6. **Contact and co-presence matrices — InVS13.** Comparison between the average matrices of link density for the contacts and the co-presence daily aggregated networks. Values are averaged over all days of the data collection. Both plots have the same colour scale.

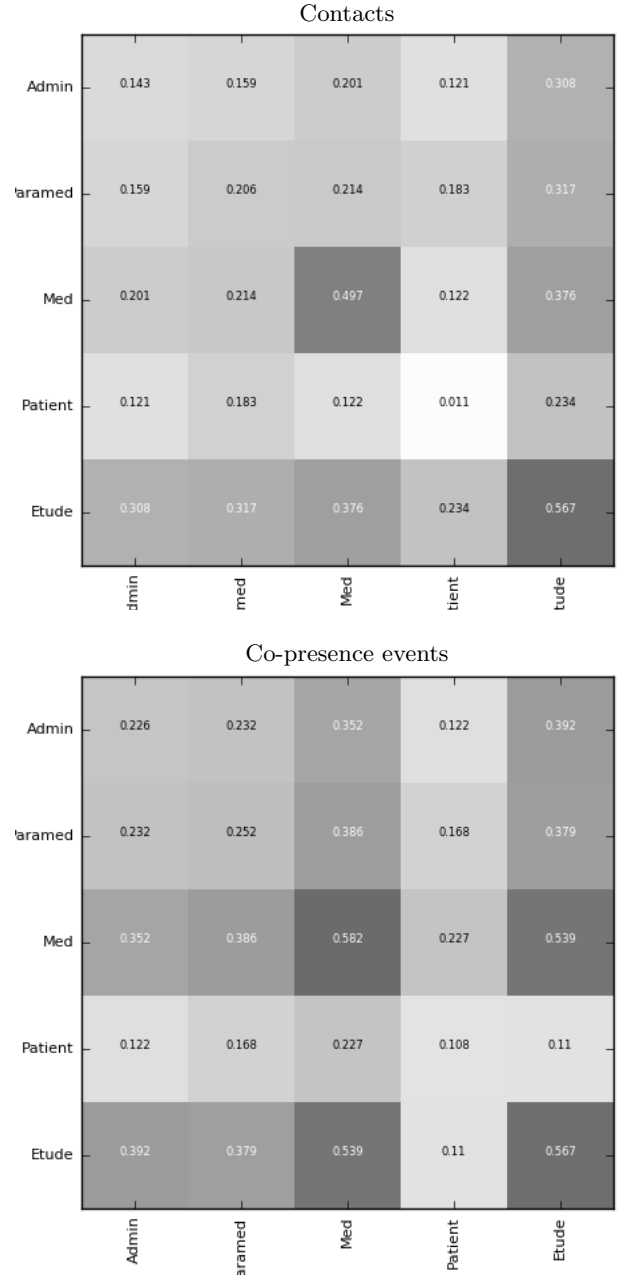

FIG. 7. **Contact and co-presence matrices — LH10.** Comparison between the average matrices of link density for the contacts and the co-presence daily aggregated networks. Values are averaged over all days of the data collection. Both plots have the same colour scale.

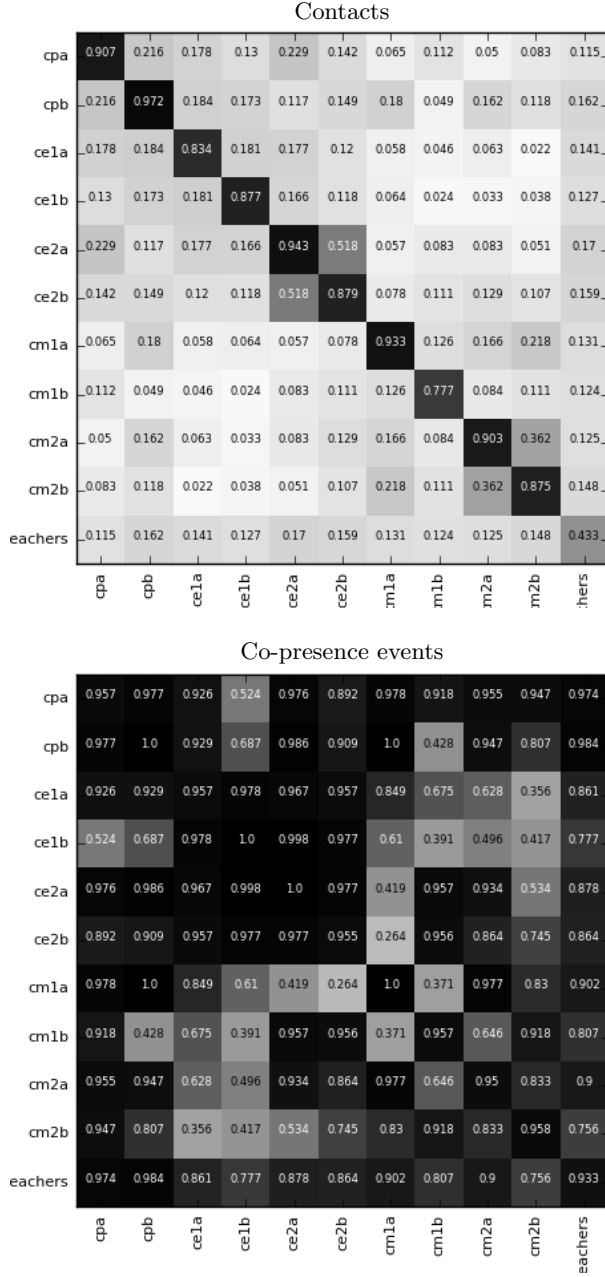

FIG. 8. **Contact and co-presence matrices — Lyon-School.** Comparison between the average matrices of link density for the contacts and the co-presence daily aggregated networks. Values are averaged over all days of the data collection. Both plots have the same colour scale.

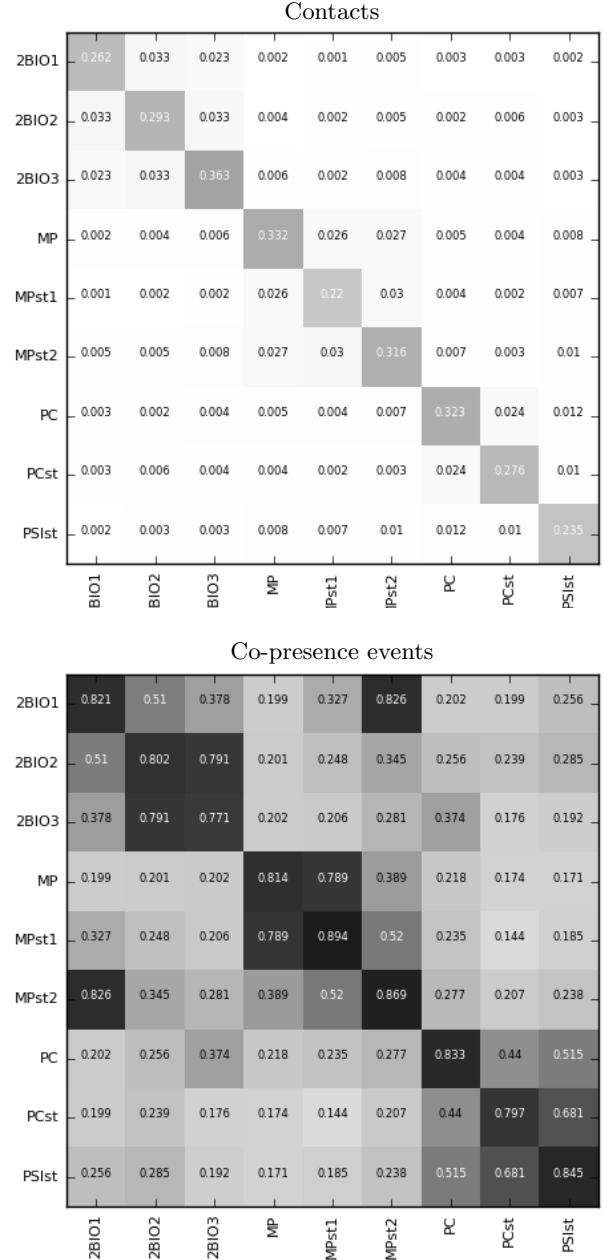

FIG. 9. **Contact and co-presence matrices — Thiers13.** Comparison between the average matrices of link density for the contacts and the co-presence daily aggregated networks. Values are averaged over all days of the data collection. Both plots have the same colour scale.

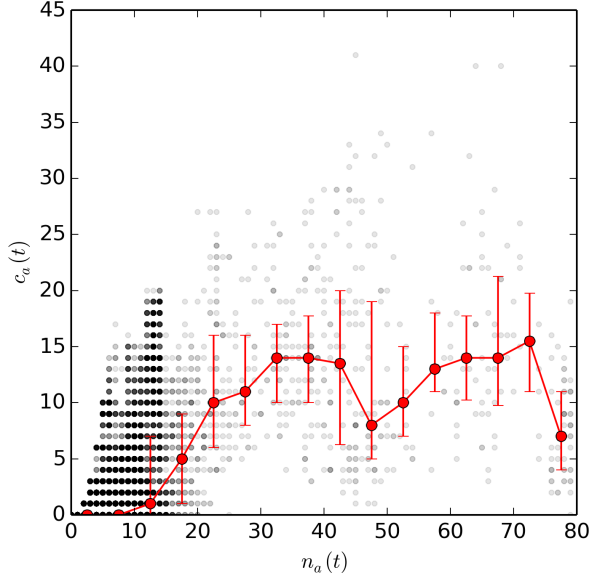

FIG. 10. Number of contacts as a function of the number of individuals present — **InVS13**. We plot the number of contacts  $c_a(t)$  occurring at time  $t$  in a certain area  $a$  as a function of the number of individuals  $n_a(t)$  present at the same time in  $a$ . The red line shows the median of the scatter plot, with error bars defined by the 25 % and 75 % percentiles.

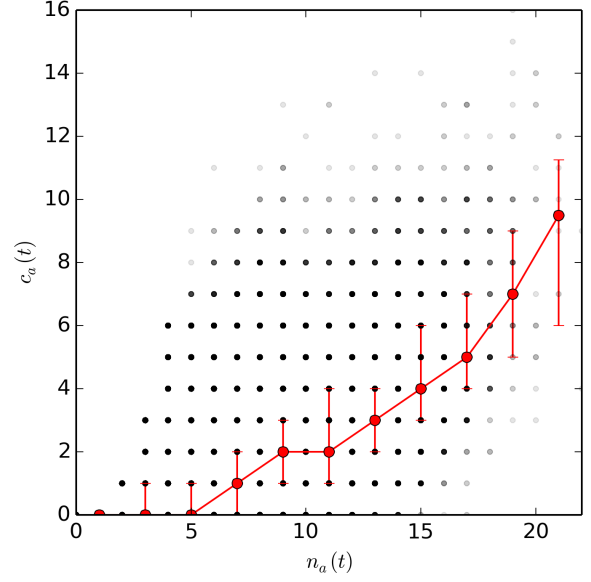

FIG. 11. Number of contacts as a function of the number of individuals present — **LH10**. We plot the number of contacts  $c_a(t)$  occurring at time  $t$  in a certain area  $a$  as a function of the number of individuals  $n_a(t)$  present at the same time in  $a$ . The red line shows the median of the scatter plot, with error bars defined by the 25 % and 75 % percentiles.

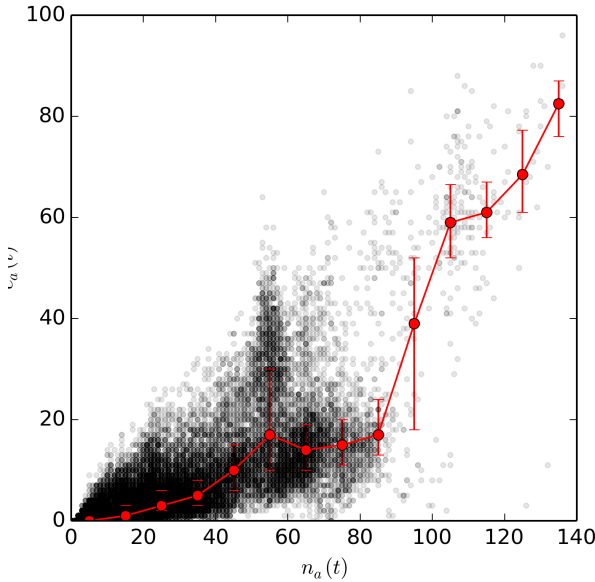

FIG. 12. Number of contacts as a function of the number of individuals present — **LyonSchool**. We plot the number of contacts  $c_a(t)$  occurring at time  $t$  in a certain area  $a$  as a function of the number of individuals  $n_a(t)$  present at the same time in  $a$ . The red line shows the median of the scatter plot, with error bars defined by the 25 % and 75 % percentiles.

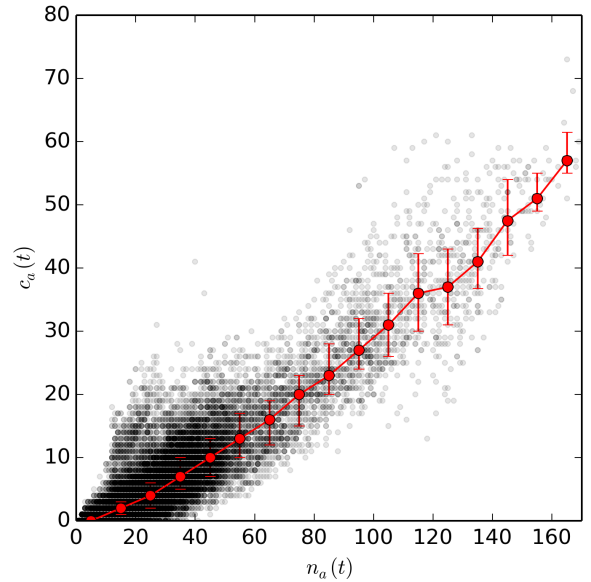

FIG. 13. Number of contacts as a function of the number of individuals present — **SFHH**. We plot the number of contacts  $c_a(t)$  occurring at time  $t$  in a certain area  $a$  as a function of the number of individuals  $n_a(t)$  present at the same time in  $a$ . The red line shows the median of the scatter plot, with error bars defined by the 25 % and 75 % percentiles.

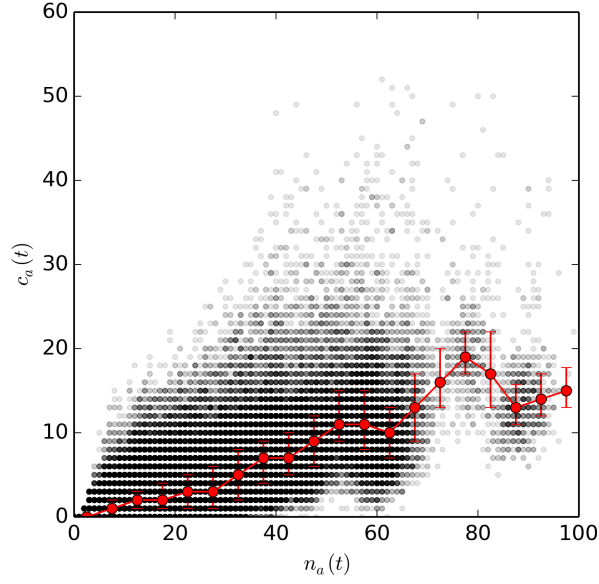

FIG. 14. Number of contacts as a function of the number of individuals present — Thiers13. We plot the number of contacts  $c_a(t)$  occurring at time  $t$  in a certain area  $a$  as a function of the number of individuals  $n_a(t)$  present at the same time in  $a$ . The red line shows the median of the scatter plot, with error bars defined by the 25 % and 75 % percentiles.

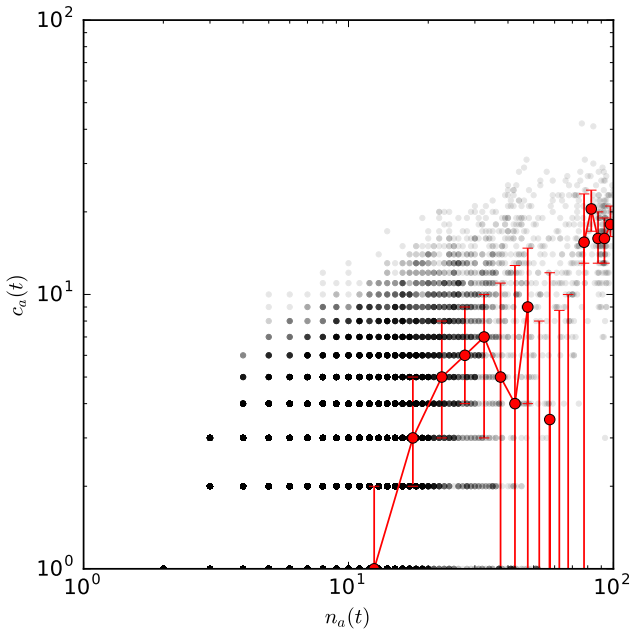

FIG. 15. Number of contacts as a function of the number of individuals present (loglog) — InVS15.

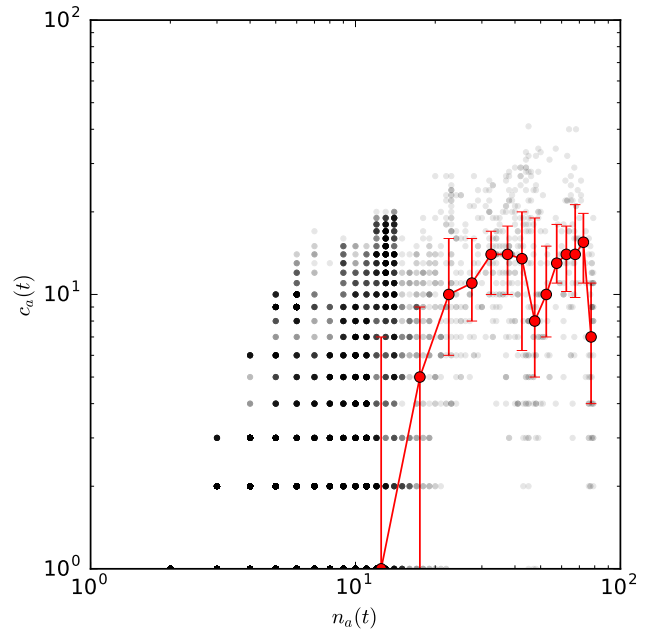

FIG. 16. Number of contacts as a function of the number of individuals present (loglog) — InVS13.



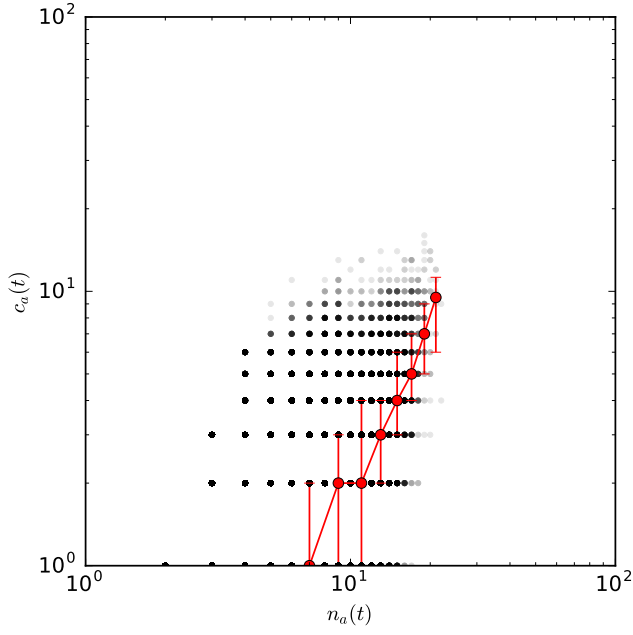

FIG. 17. Number of contacts as a function of the number of individuals present (loglog) — LH10.

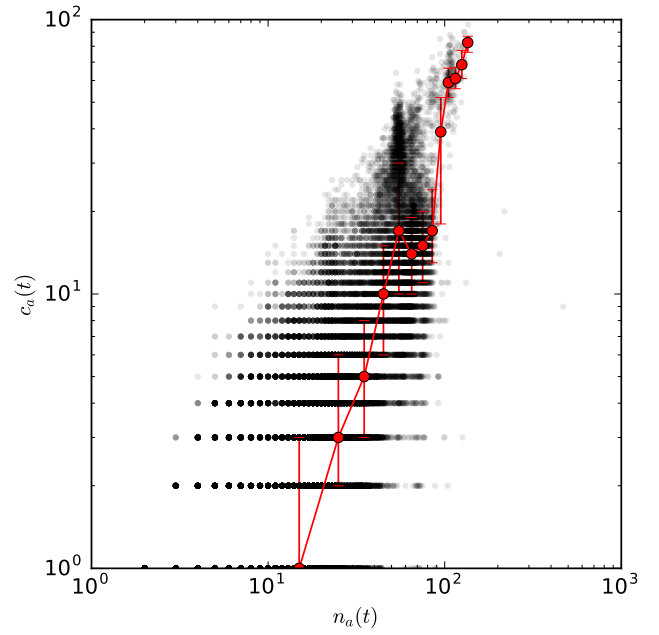

FIG. 18. Number of contacts as a function of the number of individuals present (loglog) — LyonSchool.

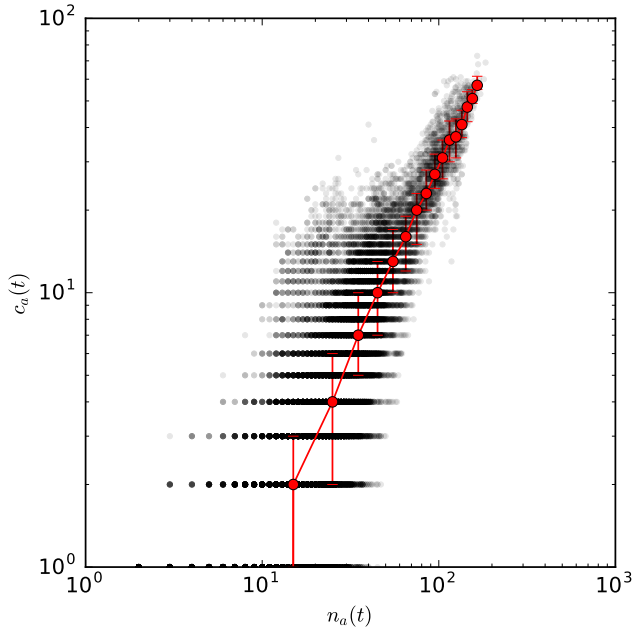

FIG. 19. Number of contacts as a function of the number of individuals present (loglog) — SFHH.

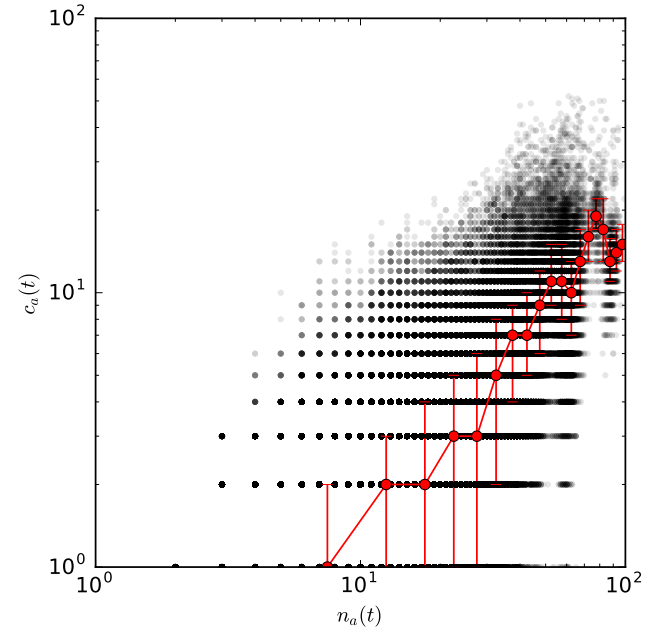

FIG. 20. Number of contacts as a function of the number of individuals present (loglog) — Thiers13.

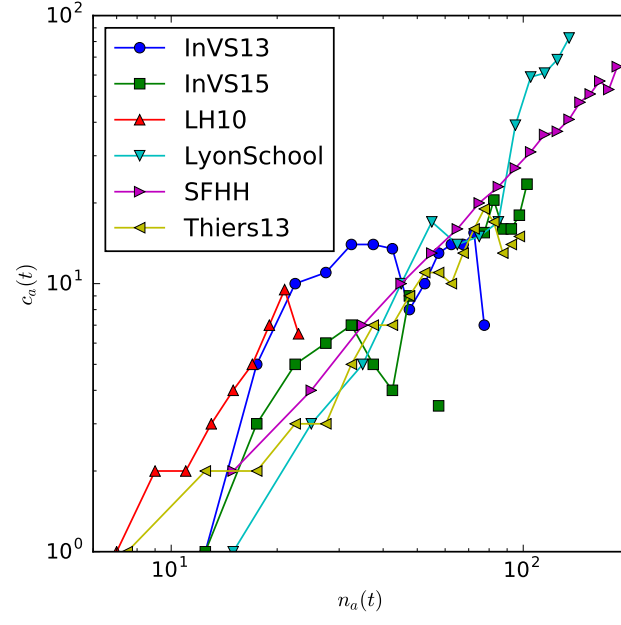

FIG. 21. Number of contacts as a function of the number of individuals present (loglog) — All data sets.

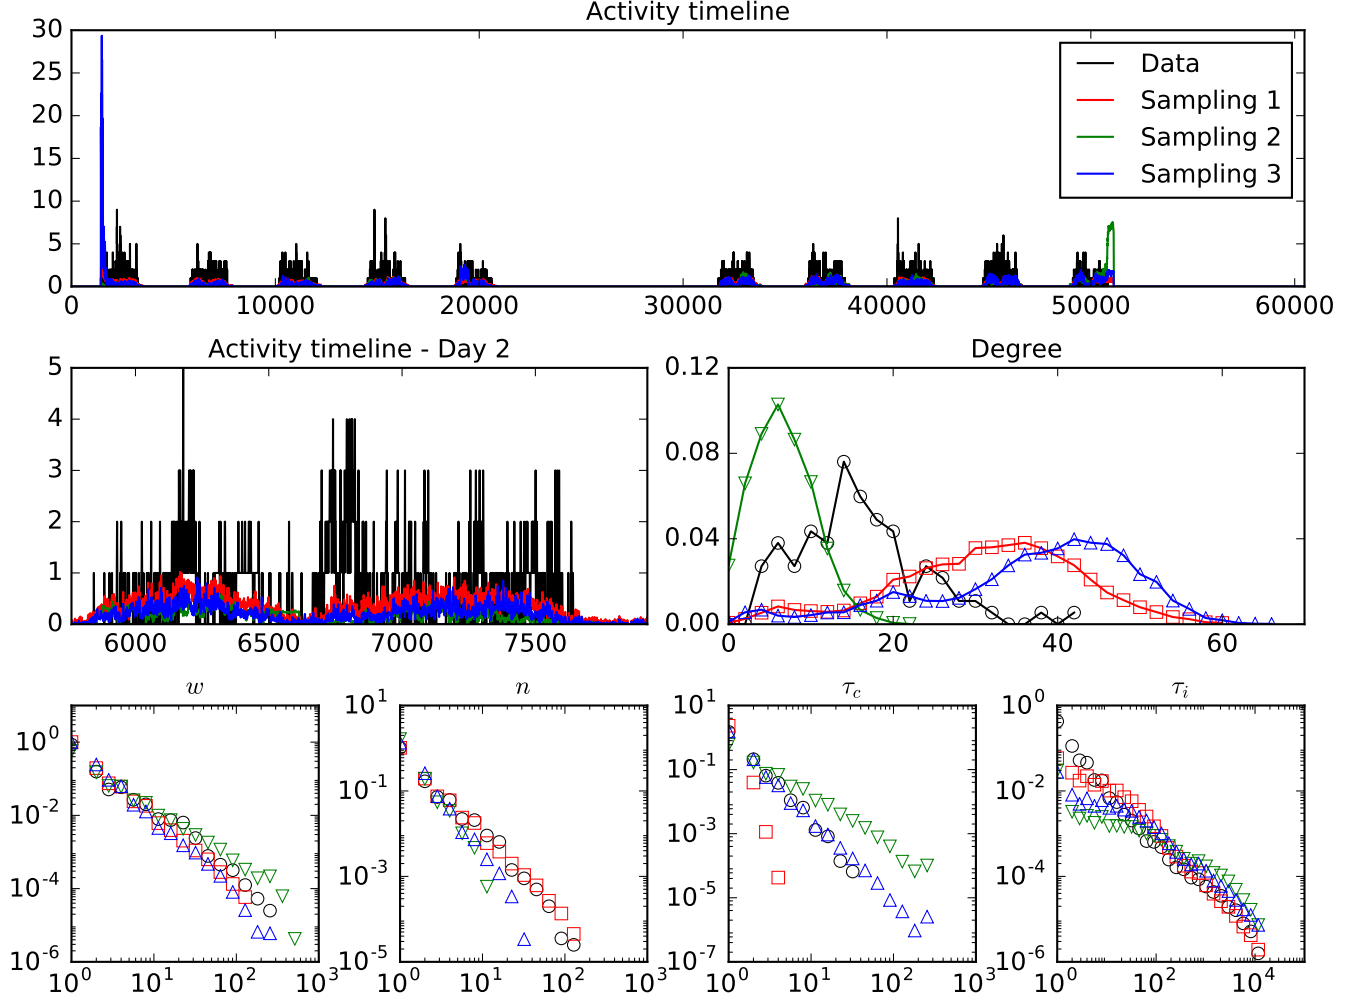

FIG. 22. **Properties of the sampled co-presence networks — InVS13.** We compare several properties of the contact network from the original data set with the surrogate contacts obtained by sampling of the co-presence data: overall timeline of contact activity, distributions of degree, weight  $w$  and number of contacts per link  $n$  in the network aggregated over the whole data collection period, and distributions of the contact duration  $\tau_c$  and inter-contact duration  $\tau_i$ .

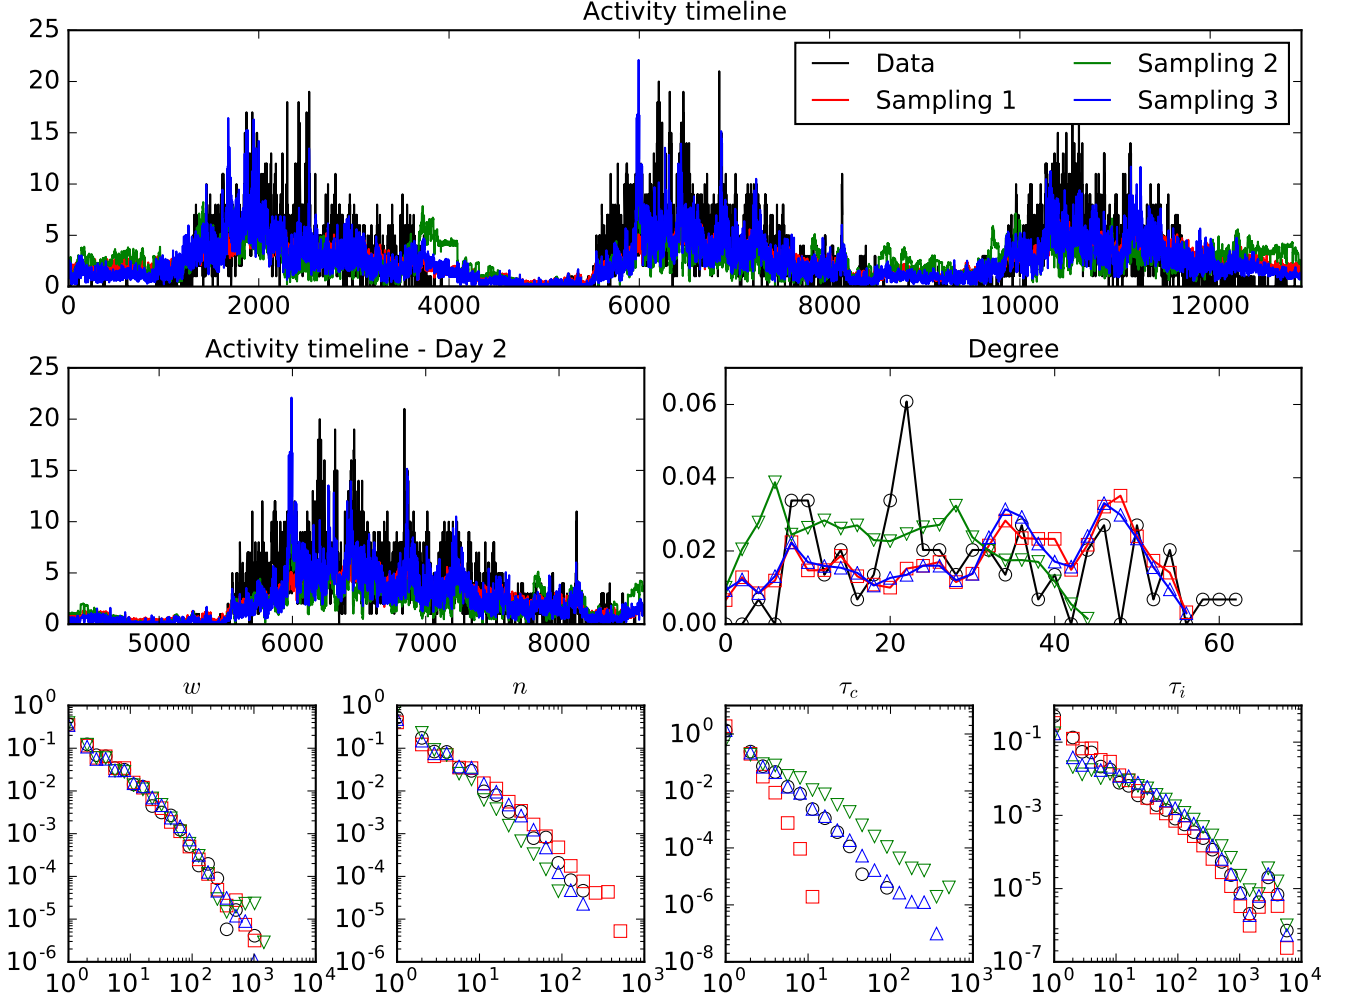

FIG. 23. **Properties of the sampled co-presence networks — LH10.** We compare several properties of the contact network from the original data set with the surrogate contacts obtained by sampling of the co-presence data: overall timeline of contact activity, distributions of degree, weight  $w$  and number of contacts per link  $n$  in the network aggregated over the whole data collection period, and distributions of the contact duration  $\tau_c$  and inter-contact duration  $\tau_i$ .

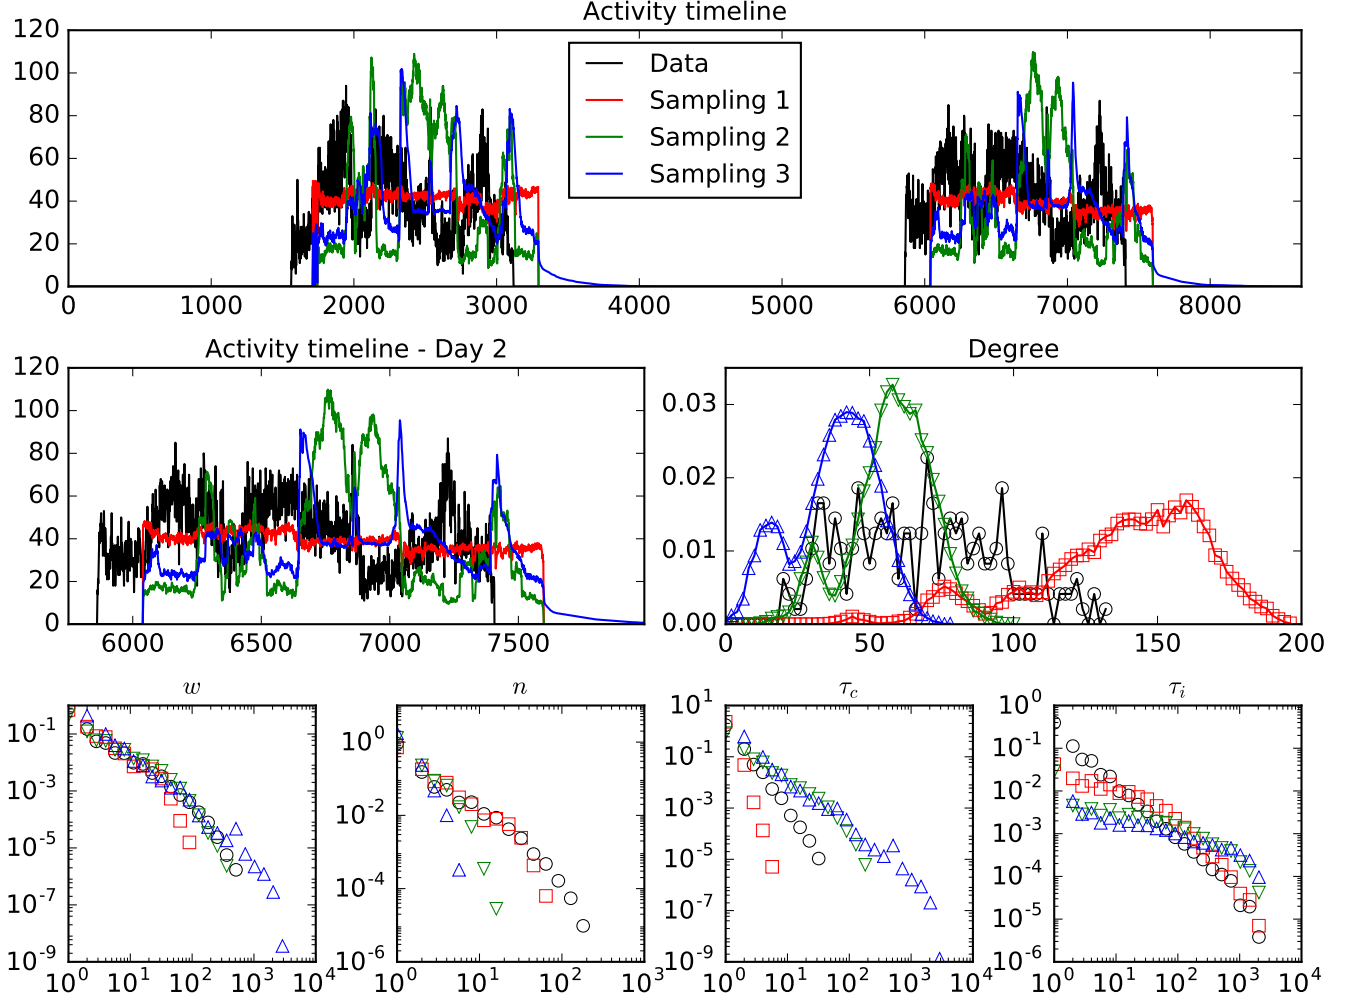

FIG. 24. **Properties of the sampled co-presence networks — LyonSchool.** We compare several properties of the contact network from the original data set with the surrogate contacts obtained by sampling of the co-presence data: overall timeline of contact activity, distributions of degree, weight  $w$  and number of contacts per link  $n$  in the network aggregated over the whole data collection period, and distributions of the contact duration  $\tau_c$  and inter-contact duration  $\tau_i$ .

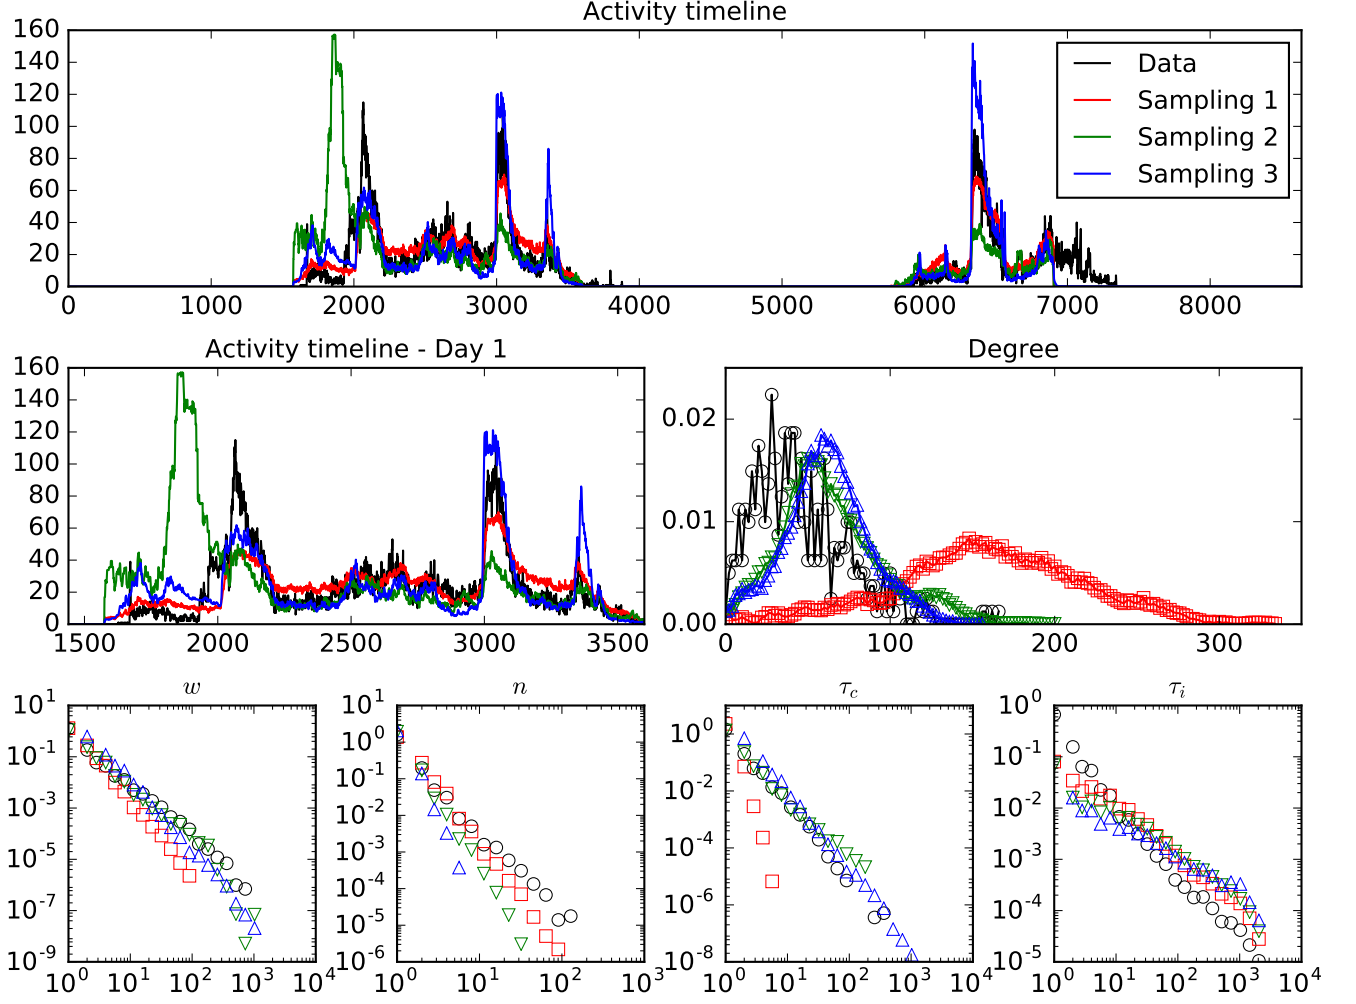

FIG. 25. **Properties of the sampled co-presence networks — SFHH.** We compare several properties of the contact network from the original data set with the surrogate contacts obtained by sampling of the co-presence data: overall timeline of contact activity, distributions of degree, weight  $w$  and number of contacts per link  $n$  in the network aggregated over the whole data collection period, and distributions of the contact duration  $\tau_c$  and inter-contact duration  $\tau_i$ .

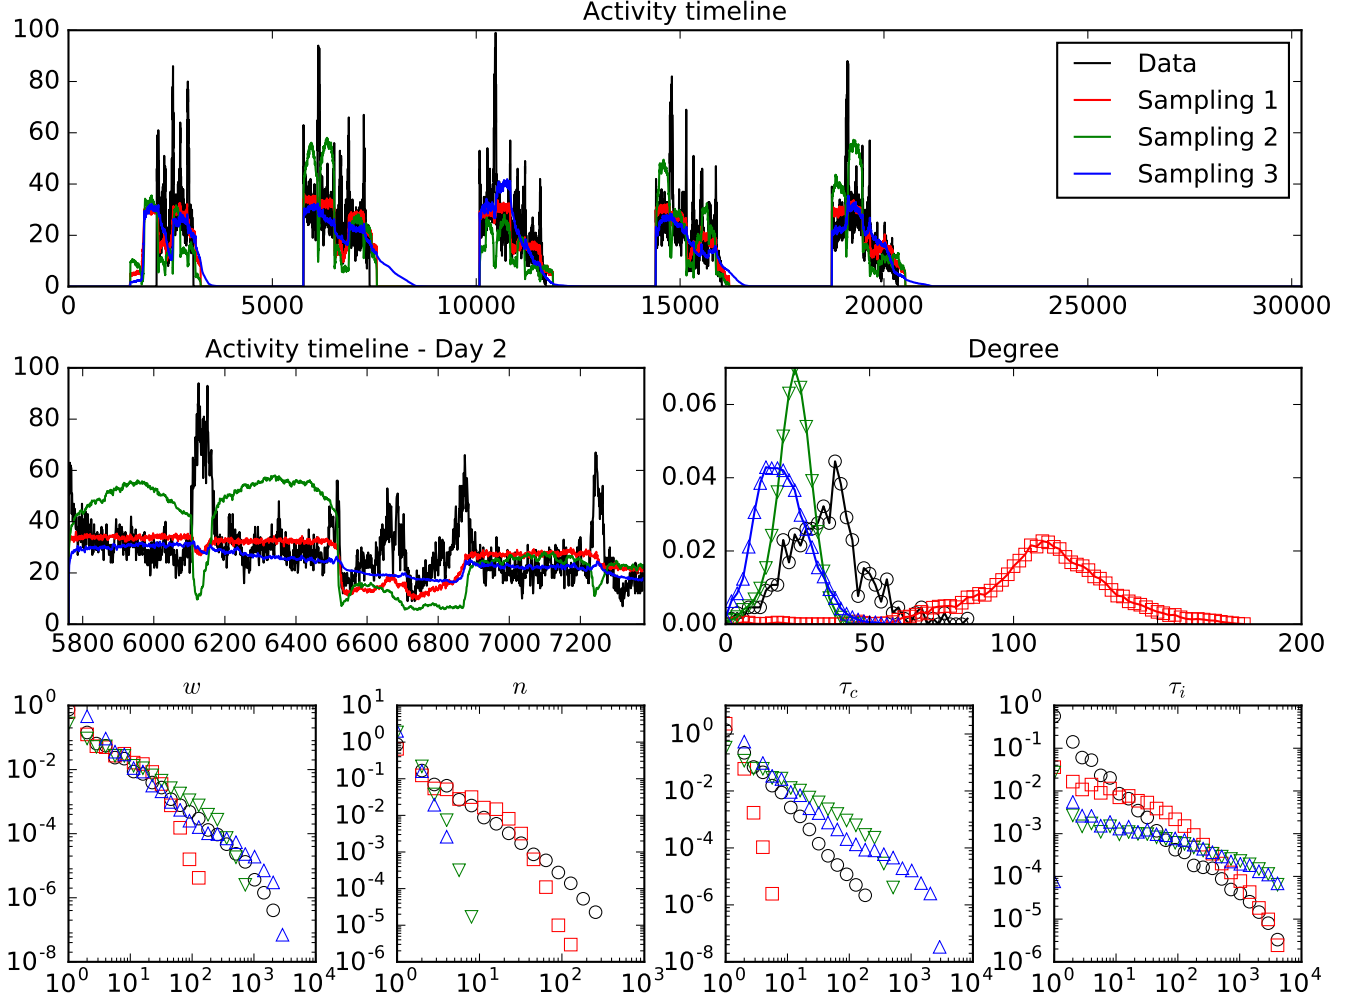

FIG. 26. **Properties of the sampled co-presence networks — Thiers13.** We compare several properties of the contact network from the original data set with the surrogate contacts obtained by sampling of the co-presence data: overall timeline of contact activity, distributions of degree, weight  $w$  and number of contacts per link  $n$  in the network aggregated over the whole data collection period, and distributions of the contact duration  $\tau_c$  and inter-contact duration  $\tau_i$ .

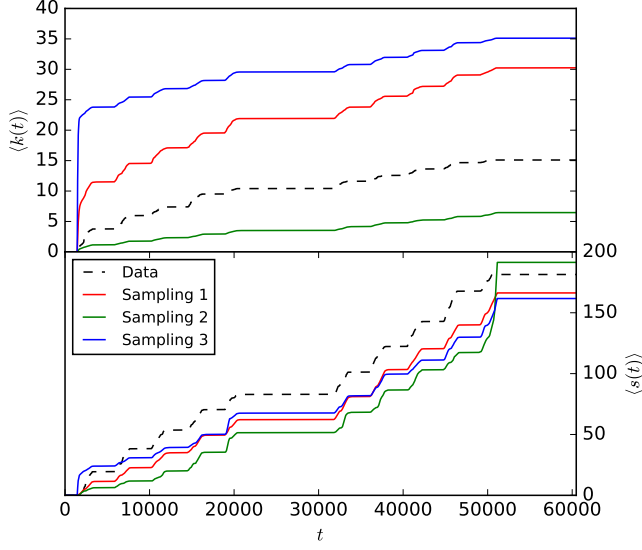

FIG. 27. **Evolution of the mean aggregated degree and strength.** We compare how the average degree  $\langle k(t) \rangle$  and the average strength  $\langle s(t) \rangle$  grow as we aggregate the network along time, for the real contact data and each sampling method. InVS13 dataset.

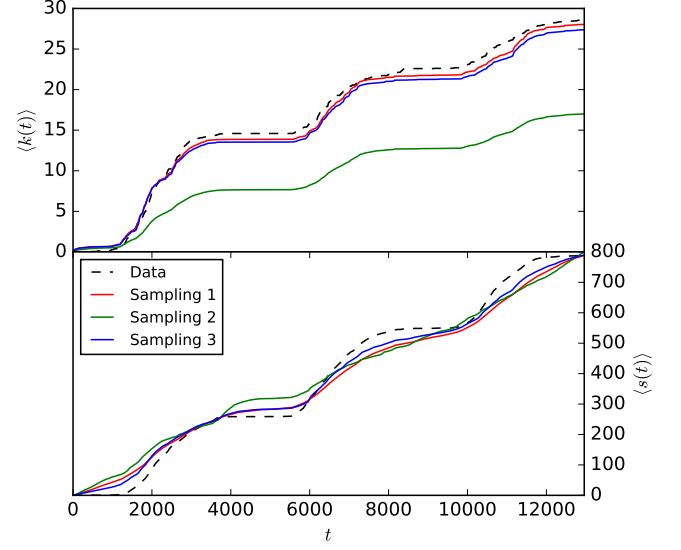

FIG. 28. **Evolution of the mean aggregated degree and strength.** We compare how the average degree  $\langle k(t) \rangle$  and the average strength  $\langle s(t) \rangle$  grow as we aggregate the network along time, for the real contact data and each sampling method. LH10 dataset.

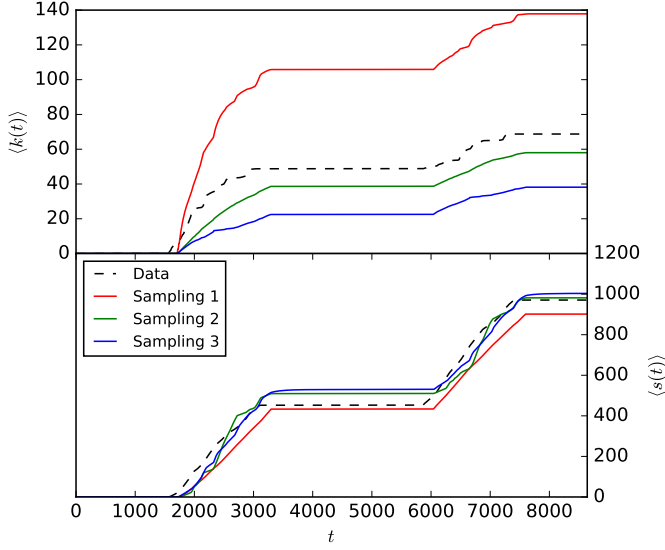

FIG. 29. **Evolution of the mean aggregated degree and strength.** We compare how the average degree  $\langle k(t) \rangle$  and the average strength  $\langle s(t) \rangle$  grow as we aggregate the network along time, for the real contact data and each sampling method. LyonSchool dataset.

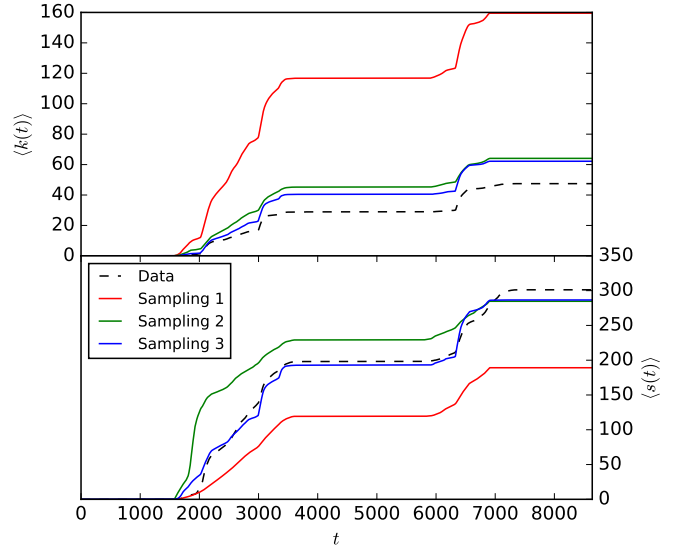

FIG. 30. **Evolution of the mean aggregated degree and strength.** We compare how the average degree  $\langle k(t) \rangle$  and the average strength  $\langle s(t) \rangle$  grow as we aggregate the network along time, for the real contact data and each sampling method. SFHH dataset.



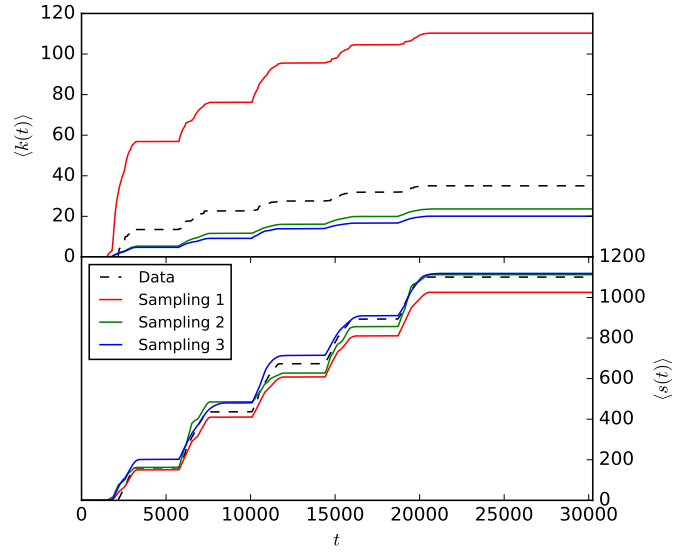

FIG. 31. **Evolution of the mean aggregated degree and strength.** We compare how the average degree  $\langle k(t) \rangle$  and the average strength  $\langle s(t) \rangle$  grow as we aggregate the network along time, for the real contact data and each sampling method. Thiers13 dataset.

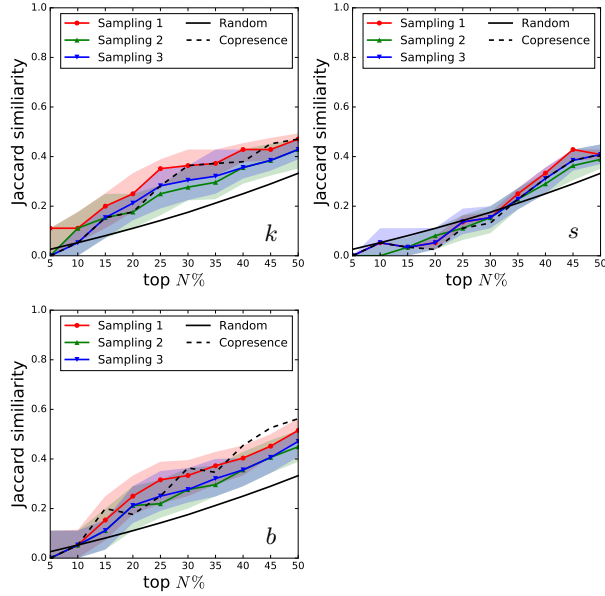

FIG. 32. **Node ranking similarity.** We plot for each model the Jaccard similarity between the top  $N\%$  nodes, ranked according to their degree  $k$ , their strength  $s$ , their betweenness centrality  $b$ , as function of  $N$ . The plot shows the median similarity and the 90 % confidence interval. InVS13 dataset.

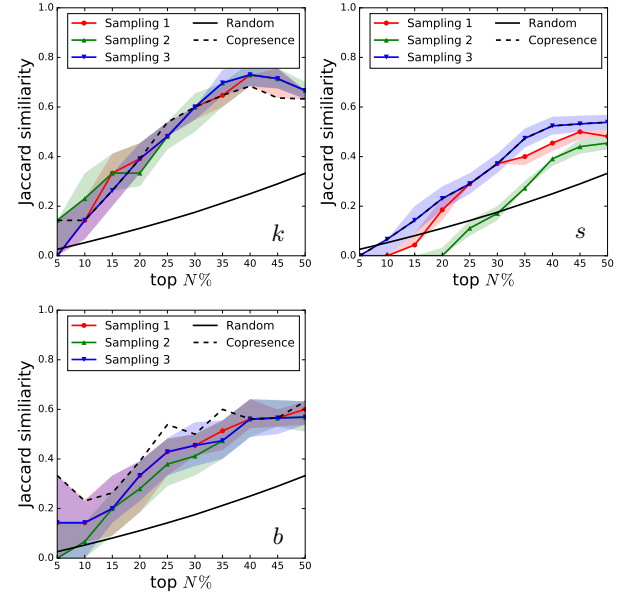

FIG. 33. **Node ranking similarity.** We plot for each model the Jaccard similarity between the top  $N\%$  nodes, ranked according to their degree  $k$ , their strength  $s$ , their betweenness centrality  $b$ , as function of  $N$ . The plot shows the median similarity and the 90 % confidence interval. LH10 dataset.

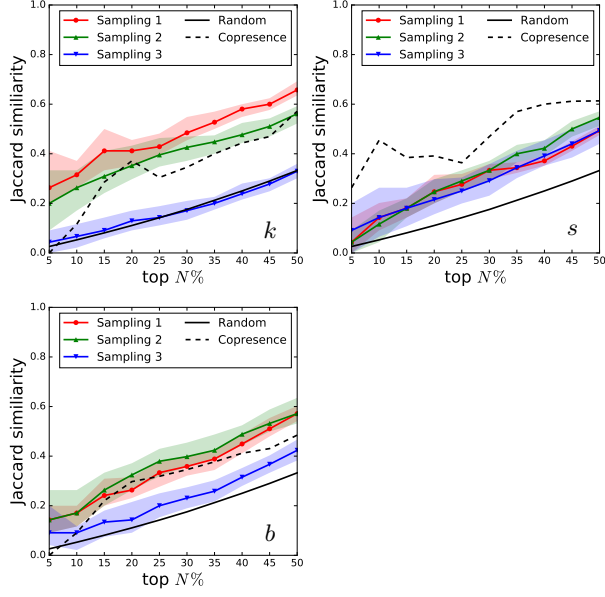

FIG. 34. **Node ranking similarity.** We plot for each model the Jaccard similarity between the top  $N\%$  nodes, ranked according to their degree  $k$ , their strength  $s$ , their betweenness centrality  $b$ , as function of  $N$ . The plot shows the median similarity and the 90 % confidence interval. LyonSchool dataset.

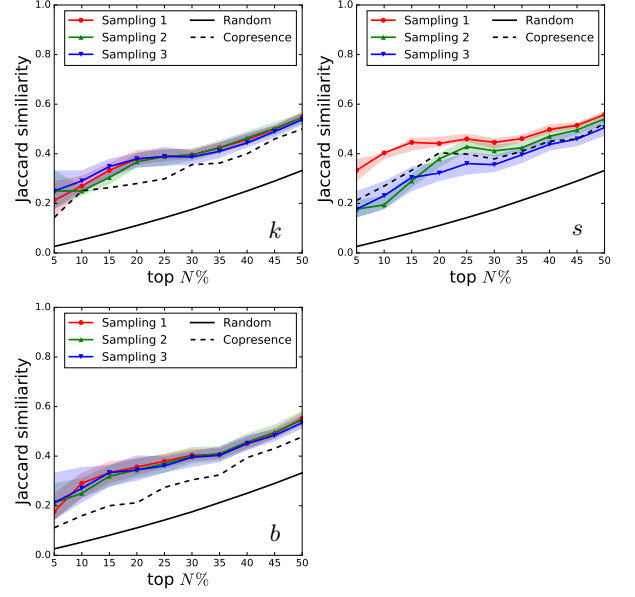

FIG. 35. **Node ranking similarity.** We plot for each model the Jaccard similarity between the top  $N\%$  nodes, ranked according to their degree  $k$ , their strength  $s$ , their betweenness centrality  $b$ , as function of  $N$ . The plot shows the median similarity and the 90 % confidence interval. SFHH dataset.

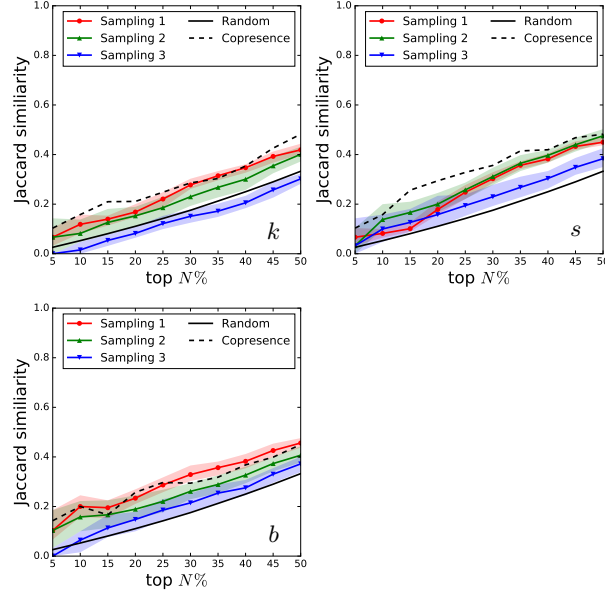

FIG. 36. **Node ranking similarity.** We plot for each model the Jaccard similarity between the top  $N\%$  nodes, ranked according to their degree  $k$ , their strength  $s$ , their betweenness centrality  $b$ , as function of  $N$ . The plot shows the median similarity and the 90 % confidence interval. Thiers13 dataset.

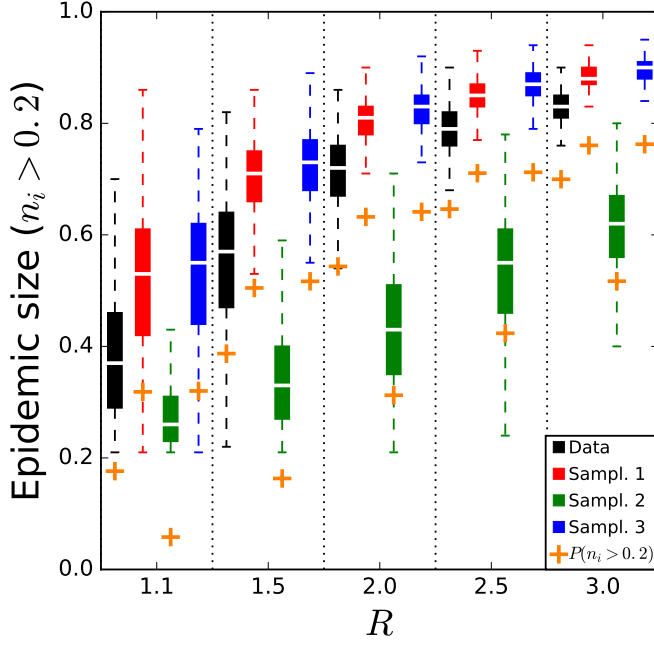

FIG. 37. **Epidemic prevalence.** We plot the fraction of the total number of outbreaks that reach at least 20% of the population (crosses) and the distribution of the sizes of these outbreaks (boxplots) as functions of the reproductive number  $R$ , for the original data and the sampled co-presence networks — InVS13 case.

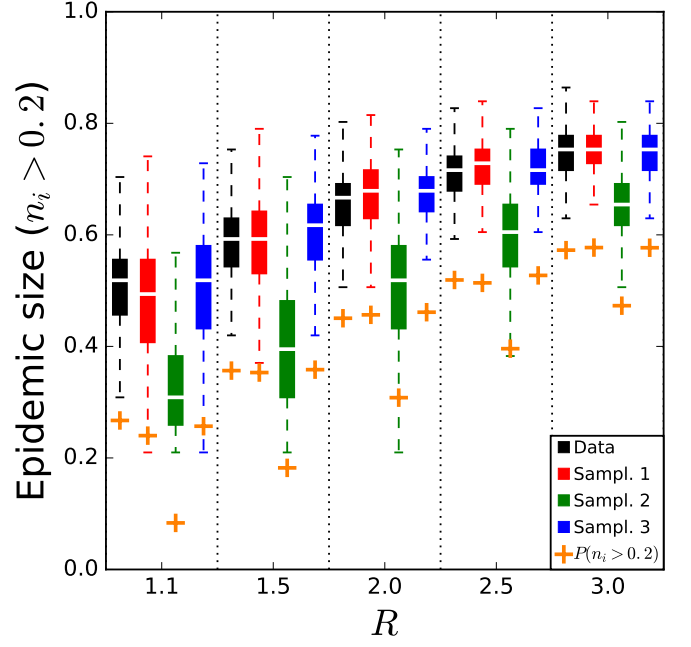

FIG. 38. **Epidemic prevalence.** We plot the fraction of the total number of outbreaks that reach at least 20% of the population (crosses) and the distribution of the sizes of these outbreaks (boxplots) as functions of the reproductive number  $R$ , for the original data and the sampled co-presence networks — LH10 case.

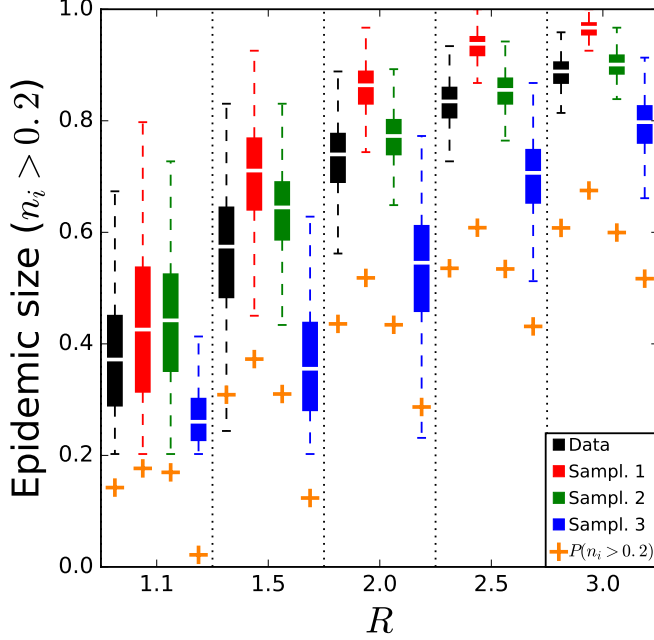

FIG. 39. **Epidemic prevalence.** We plot the fraction of the total number of outbreaks that reach at least 20% of the population (crosses) and the distribution of the sizes of these outbreaks (boxplots) as functions of the reproductive number  $R$ , for the original data and the sampled co-presence networks — LyonSchool case.

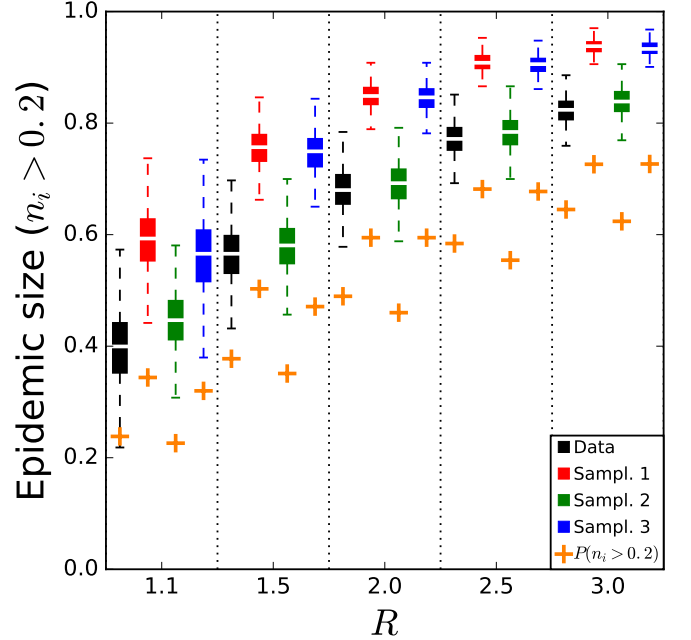

FIG. 40. **Epidemic prevalence.** We plot the fraction of the total number of outbreaks that reach at least 20% of the population (crosses) and the distribution of the sizes of these outbreaks (boxplots) as functions of the reproductive number  $R$ , for the original data and the sampled co-presence networks — SFHH case.

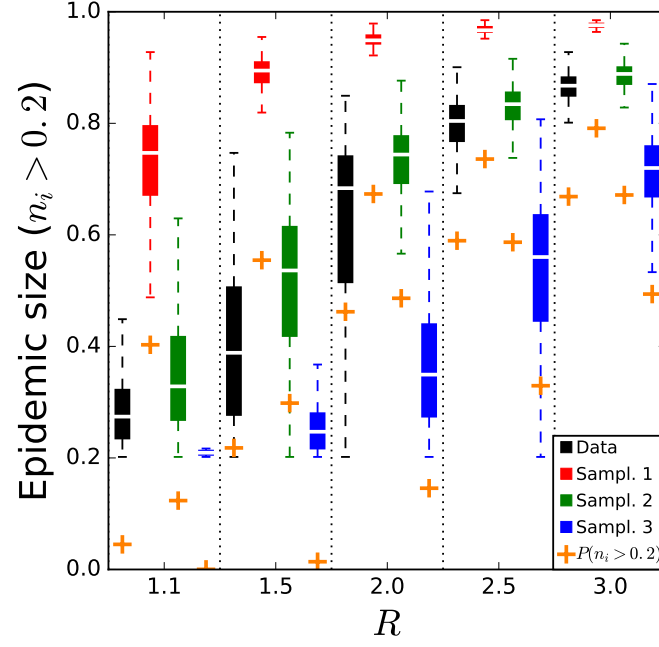

FIG. 41. **Epidemic prevalence.** We plot the fraction of the total number of outbreaks that reach at least 20 % of the population (crosses) and the distribution of the sizes of these outbreaks (boxplots) as functions of the reproductive number  $R$ , for the original data and the sampled co-presence networks — Thiers13 case.

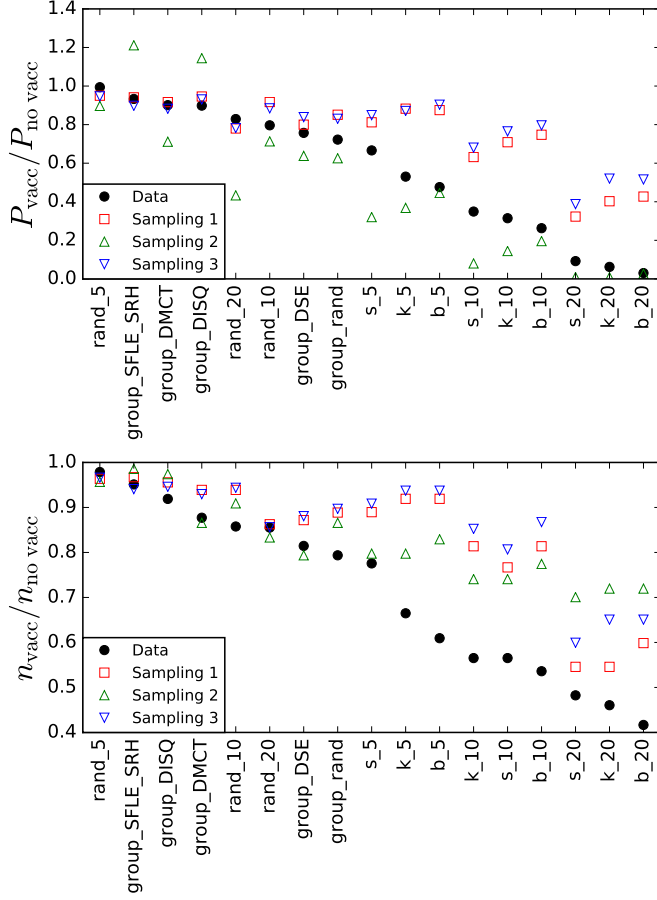

FIG. 42. **Vaccination strategies.** We plot the ratio between the vaccination and no vaccination cases of the fraction of the total number of outbreaks that reach at least 20% of the population (top), and of the median size of these outbreaks (bottom) for different vaccination strategies, for the original data and the reconstructed networks. The *group\_n* strategies consist in vaccinating one or several groups entirely; the *group\_rand* strategy vaccinates  $n_g$  random nodes, where  $n_g$  is the average group size; the *rand\_n* strategies randomly vaccinates a specified fraction of nodes; the *b\_n*, *k\_n*, *s\_n* strategies vaccinate the top  $n\%$  nodes according to, respectively, betweenness centrality, degree and strength ranking. InVS13 case.

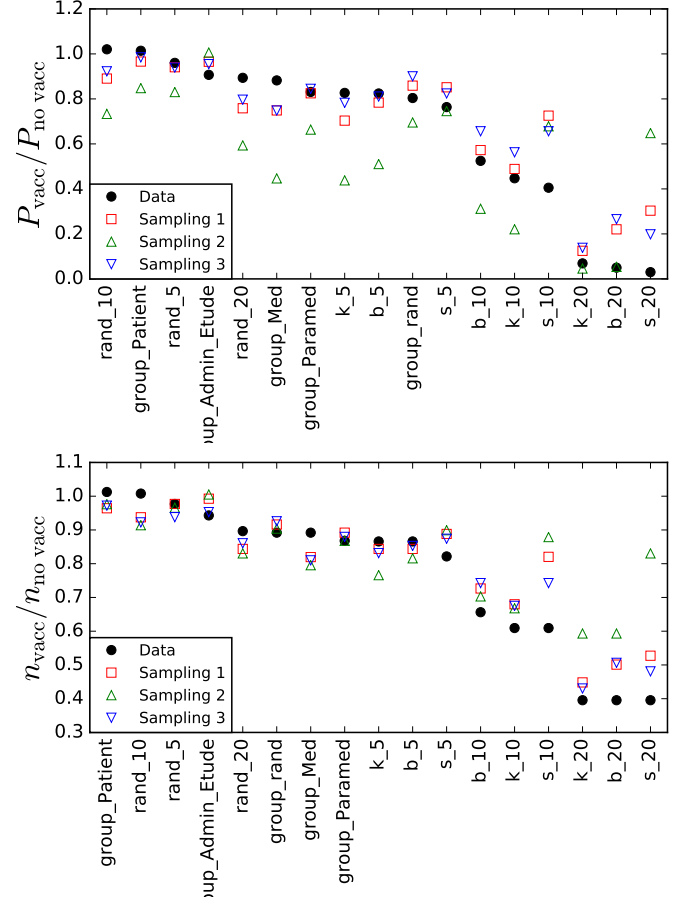

FIG. 43. **Vaccination strategies.** We plot the ratio between the vaccination and no vaccination cases of the fraction of the total number of outbreaks that reach at least 20% of the population (top), and of the median size of these outbreaks (bottom) for different vaccination strategies, for the original data and the reconstructed networks. The *group\_n* strategies consist in vaccinating one or several groups entirely; the *group\_rand* strategy vaccinates  $n_g$  random nodes, where  $n_g$  is the average group size; the *rand\_n* strategies randomly vaccinates a specified fraction of nodes; the *b\_n*, *k\_n*, *s\_n* strategies vaccinate the top  $n\%$  nodes according to, respectively, betweenness centrality, degree and strength ranking. LH10 case.



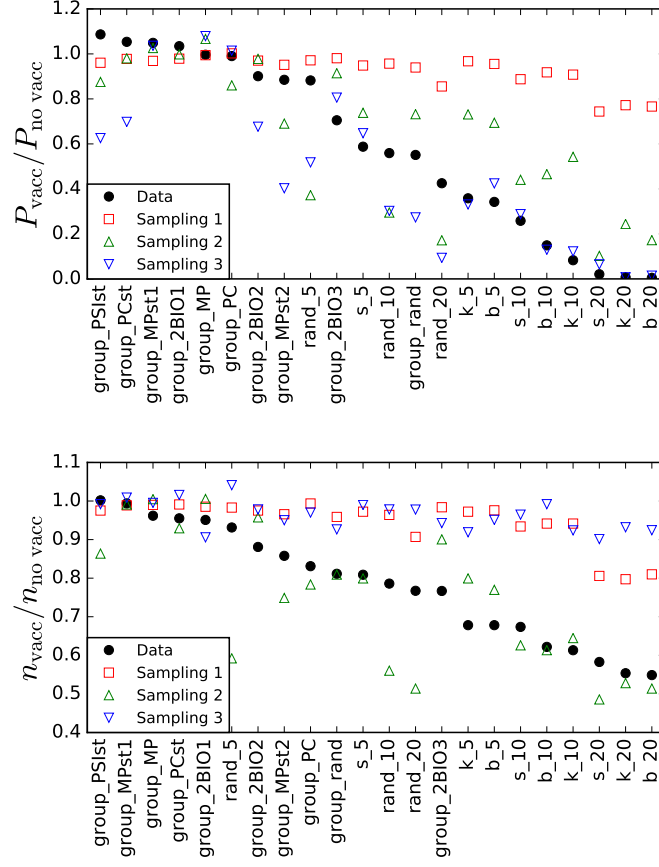

FIG. 46. **Vaccination strategies.** We plot the ratio between the vaccination and no vaccination cases of the fraction of the total number of outbreaks that reach at least 20% of the population (top), and of the median size of these outbreaks (bottom) for different vaccination strategies, for the original data and the reconstructed networks. The *group\_n* strategies consist in vaccinating one or several groups entirely; the *group\_rand* strategy vaccinates  $n_g$  random nodes, where  $n_g$  is the average group size; the *rand\_n* strategies randomly vaccinates a specified fraction of nodes; the *b\_n*, *k\_n*, *s\_n* strategies vaccinate the top  $n\%$  nodes according to, respectively, betweenness centrality, degree and strength ranking. Thiers13 case.
